# Supplementary material for: Intrinsic Nonlinear Planar Hall Effect
Source: arXiv:2208.03639 source file (2022-08-07)
Supplement: Supplementary file 1 [file NLPHE_Supp.pdf]

# Supplemental Material for Intrinsic Nonlinear Planar Hall Effect

## CONTENTS

I. Theory for intrinsic nonlinear planar Hall effect 1
A. General formulation 1
B. Nonlinear intrinsic planar Hall effect 2

II. First-principles calculation of Janus monolayer 3

References 3

## I. THEORY FOR INTRINSIC NONLINEAR PLANAR HALL EFFECT

### A. General formulation

The Hamiltonian felt by a narrow wave packet [1] reads $\hat{H} = \hat{H}_c + \hat{H}'$, where $\hat{H}_c = \hat{H}_0 + \frac{g}{\hbar}\mu_{\rm B}\hat{\mathbf{s}}\cdot\mathbf{B} - e\phi(\mathbf{r}_c)$ is the local Hamiltonian and $\hat{H}' = e\mathbf{E}\cdot(\hat{\mathbf{r}} - \mathbf{r}_c)$. Here $\hat{H}_0$ is the genuine Hamiltonian for a periodic crystal, $\phi$ is the slowly varying electrostatic potential and is expanded around the wave packet center $\boldsymbol{r}_c$, and $\mathbf{E} = -\nabla\phi$ is the electric field. We are interested in the transverse charge current response at the second order of $E$ field in two-dimensional electronic systems subject to an in-plane uniform magnetic field $\mathbf{B}$, i.e., the second order nonlinear planar Hall effect. The magnetic field couples to the electron spin $\hat{\mathbf{s}}$ hence enters into the Bloch wave function $e^{i\boldsymbol{k}\cdot\hat{\boldsymbol{r}}}|\tilde{u}_{n\boldsymbol{k}}\rangle$ and band energy $\tilde{\varepsilon}_{n\boldsymbol{k}} = \langle\tilde{u}_{n\boldsymbol{k}}|[\hat{H}_0(\boldsymbol{k}) + \frac{g}{\hbar}\mu_{\rm B}\hat{\mathbf{s}}\cdot\mathbf{B}]|\tilde{u}_{n\boldsymbol{k}}\rangle$. Here $n$ and $\hbar\boldsymbol{k}$ are the band index and crystal momentum, respectively.

We formulate the transport theory accurate to the second order of $E$ field on the basis of the Bloch state of the local Hamiltonian $\hat{H}_c$ [1, 2]. The equations of motion read (we set $e = \hbar = 1$)

$$\dot{\boldsymbol{r}}_c = \frac{\partial(\tilde{\varepsilon} + \delta\tilde{\varepsilon})}{\partial\boldsymbol{k}} + \boldsymbol{E}\times(\tilde{\boldsymbol{\Omega}} + \delta^{\rm E}\tilde{\boldsymbol{\Omega}}), \quad (1)$$

where $\tilde{\boldsymbol{\Omega}}_n(\boldsymbol{k}) = \partial_{\boldsymbol{k}}\times\tilde{\boldsymbol{\mathcal{A}}}_n(\boldsymbol{k})$ is the Berry curvature derivable from the Berry connection $\tilde{\mathcal{A}}_n(\boldsymbol{k}) = \langle\tilde{u}_{n\boldsymbol{k}}|i\partial_{\boldsymbol{k}}|\tilde{u}_{n\boldsymbol{k}}\rangle$ in the zeroth order of the $E$ field, and $\delta^{\rm E}\tilde{\boldsymbol{\Omega}} = \partial_{\boldsymbol{k}}\times\tilde{\boldsymbol{\mathcal{A}}}_n^E(\boldsymbol{k})$ is the Berry curvature in the first order of the $E$ field, with $\tilde{\boldsymbol{\mathcal{A}}}_n^E(\boldsymbol{k}) = 2\,{\rm Re}\langle\tilde{u}_{n\boldsymbol{k}}|i\partial_{\boldsymbol{k}}|\delta^{\rm E}\tilde{u}_{n\boldsymbol{k}}\rangle$ being the Berry connection induced by $E$ field. As $|\delta^{\rm E}\tilde{u}_{n\boldsymbol{k}}\rangle = \sum_{n_1\neq n}\frac{\boldsymbol{E}\cdot\tilde{\mathcal{A}}_{n_1 n}(\boldsymbol{k})}{\tilde{\varepsilon}_{n\boldsymbol{k}} - \tilde{\varepsilon}_{n_1\boldsymbol{k}}}|\tilde{u}_{n_1\boldsymbol{k}}\rangle$, we have $(\tilde{\mathcal{A}}_n^E)_a \equiv \tilde{G}_{ab}^n E_b$, with the Berry connection polarizability (BCP)

$$\tilde{G}_{ab}^n = 2{\rm Re}\sum_{n_1\neq n}\frac{\langle\tilde{u}_{n\boldsymbol{k}}|\hat{v}_a|\tilde{u}_{n_1\boldsymbol{k}}\rangle\langle\tilde{u}_{n_1\boldsymbol{k}}|\hat{v}_b|\tilde{u}_{n\boldsymbol{k}}\rangle}{(\tilde{\varepsilon}_n - \tilde{\varepsilon}_{n_1})^3}. \quad (2)$$

Besides, the wave packet energy up to the second order of the electric field is given by $\delta\tilde{\varepsilon}_{n\mathbf{k}} = -\frac{1}{2}\tilde{\boldsymbol{\mathcal{A}}}_n^E(\boldsymbol{k})\cdot\boldsymbol{E}$.

The charge current can be evaluated from

$$\begin{aligned}\boldsymbol{j} &= -\int[d\boldsymbol{k}]f(\tilde{\varepsilon} + \delta\tilde{\varepsilon})\left[\frac{\partial(\tilde{\varepsilon} + \delta\tilde{\varepsilon})}{\partial\boldsymbol{k}} + \boldsymbol{E}\times(\tilde{\boldsymbol{\Omega}} + \delta^{\rm E}\tilde{\boldsymbol{\Omega}})\right]\\ &= -\int[d\boldsymbol{k}]\frac{\partial g(\tilde{\varepsilon} + \delta\tilde{\varepsilon})}{\hbar\partial\boldsymbol{k}} - \int[d\boldsymbol{k}]f(\tilde{\varepsilon} + \delta\tilde{\varepsilon})\,\boldsymbol{E}\times(\tilde{\boldsymbol{\Omega}} + \delta^{\rm E}\tilde{\boldsymbol{\Omega}})\\ &= -\int[d\boldsymbol{k}]f(\tilde{\varepsilon} + \delta\tilde{\varepsilon})\,\boldsymbol{E}\times(\tilde{\boldsymbol{\Omega}} + \delta^{\rm E}\tilde{\boldsymbol{\Omega}}),\end{aligned}$$

where $[d\boldsymbol{k}]$ is shorthand for $\sum_n d^2\boldsymbol{k}/(2\pi)^2$, and $f$ is the occupation function, which is taken to be the Fermi-Dirac distribution $f(\tilde{\varepsilon} + \delta\tilde{\varepsilon})$ since we only consider the intrinsic response dictated by band structures. Note that $f(\varepsilon) = \partial g(\varepsilon)/\partial\varepsilon$, and $g(\varepsilon) = -k_B T\ln[1 + e^{-(\varepsilon-\mu)/k_B T}]$ is the grand potential density contributed by a particular Bloch state. Up to the second order in the electric field, we have

$$\boldsymbol{j} = -\boldsymbol{E}\times\int[d\boldsymbol{k}]f(\varepsilon)\,\tilde{\boldsymbol{\Omega}} - \boldsymbol{E}\times\int[d\boldsymbol{k}]f(\varepsilon)\,\delta^{\rm E}\tilde{\boldsymbol{\Omega}}, \quad (3)$$

i.e.,

$$\boldsymbol{j} = -\boldsymbol{E} \times \int [d\boldsymbol{k}] f\left(\tilde{\varepsilon}\right) \tilde{\boldsymbol{\Omega}} - \boldsymbol{E} \times \int [d\boldsymbol{k}] f\left(\tilde{\varepsilon}\right) \partial_{\boldsymbol{k}} \times \tilde{\boldsymbol{\mathcal{A}}}_n^E\left(\boldsymbol{k}\right), \tag{4}$$

These equations are amenable to first-principles and model calculations, and provide a general recipe for the intrinsic Hall current in the presence of an in-plane magnetic field. The linear-in-$E$-field term $\boldsymbol{j}^{(1)} = -\boldsymbol{E} \times \int [d\boldsymbol{k}] f\left(\tilde{\varepsilon}\right) \tilde{\boldsymbol{\Omega}}$ contains the linear anomalous Hall effect when $B = 0$ and the linear planar Hall effect when $B \neq 0$. The quadratic-in-$E$-field current

$$\boldsymbol{j}^{(2)} = -\boldsymbol{E} \times \int [d\boldsymbol{k}] f\left(\tilde{\varepsilon}\right) \partial_{\boldsymbol{k}} \times \tilde{\boldsymbol{\mathcal{A}}}_n^E\left(\boldsymbol{k}\right) \tag{5}$$

contains the second order nonlinear anomalous Hall effect when $B = 0$ and the nonlinear planar Hall effect when $B \neq 0$.

For the second order current $j_a^{(2)} = \chi_{abc}^{\text{int}} E_b E_c$, we have

$$\chi_{abc}^{\text{int}} = \int [d\boldsymbol{k}] f\left(\tilde{\varepsilon}\right) \left(\partial_b \tilde{G}_{ac} - \partial_a \tilde{G}_{bc}\right), \tag{6}$$

where $\partial_a \equiv \partial_{k_a}$.

### B. Nonlinear intrinsic planar Hall effect

We are interested in the nonlinear planar Hall effect in the linear order of the magnetic field. In the weak magnetic field semiclassical regime, we can expand the eigenstate $|\tilde{u}_{n\boldsymbol{k}}\rangle$ up to the first order of the Zeeman field:

$$|\tilde{u}_n\rangle = |u_n\rangle - \boldsymbol{B} \cdot \sum_{n' \neq n} \frac{\langle u_{n'}|\hat{\boldsymbol{\mathcal{M}}}|u_n\rangle}{\varepsilon_n - \varepsilon_{n'}} |u_{n'}\rangle, \tag{7}$$

and make use of $\tilde{\varepsilon}_n = \varepsilon_n - \boldsymbol{B} \cdot \langle u_n|\hat{\boldsymbol{\mathcal{M}}}|u_n\rangle$. Here $|u_n\rangle$ and $\varepsilon_n$ being the periodic part of the Bloch state and band energy of the zero-field Hamiltonian $\hat{H}_0$, respectively, $\hat{\boldsymbol{\mathcal{M}}} = -g\mu_B \hat{\boldsymbol{s}}$ is the operator for spin magnetic moment. $\tilde{G}_{ab}^n$ can thus be decomposed into

$$\tilde{G}_{ab}^n = G_{ab}^n + \Lambda_{abc}^n B_c, \tag{8}$$

where $G_{ab}^n = 2\text{Re} \sum_{m \neq n} \frac{v_a^{nm} v_b^{mn}}{(\varepsilon_n - \varepsilon_m)^3}$ is the BCP in the absence of the Zeeman field, and

$$\Lambda_{abc}^n = 2\text{Re} \sum_{m \neq n} \left[ \frac{3 v_a^{nm} v_b^{mn} \left(\mathcal{M}_c^n - \mathcal{M}_c^m\right)}{(\varepsilon_n - \varepsilon_m)^4} - \sum_{\ell \neq n} \frac{\left(v_a^{\ell m} v_b^{mn} + v_b^{\ell m} v_a^{mn}\right) \mathcal{M}_c^{n\ell}}{\left(\varepsilon_n - \varepsilon_l\right)\left(\varepsilon_n - \varepsilon_m\right)^3} - \sum_{\ell \neq m} \frac{\left(v_a^{\ell n} v_b^{nm} + v_b^{\ell n} v_a^{nm}\right) \mathcal{M}_c^{m\ell}}{\left(\varepsilon_m - \varepsilon_l\right)\left(\varepsilon_n - \varepsilon_m\right)^3} \right] \tag{9}$$

is the spin susceptibility of BCP, which is nothing but Eq. (3) in the main text.

Gathering the above results, up to the first order of magnetic field, the second order intrinsic current response coefficient, Eq. (6), reads

$$\chi_{abc}^{\text{int}} = \chi_{abc}^{\text{int}}|_{B=0} + B_d \chi_{abcd}^{\text{int}}, \tag{10}$$

where $\chi_{abcd}^{\text{int}} \equiv \left(\partial_{B_d} \chi_{abc}^{\text{int}}\right)|_{B=0}$ is given by

$$\chi_{abcd}^{\text{int}} = -\int [d\boldsymbol{k}] \frac{\partial f\left(\varepsilon\right)}{\partial \varepsilon} \mathcal{M}_d \left(\partial_b G_{ac} - \partial_a G_{bc}\right) + \int [d\boldsymbol{k}] f\left(\varepsilon\right) \left(\partial_b \Lambda_{acd} - \partial_a \Lambda_{bcd}\right), \tag{11}$$

just Eq. (5) in the main text.

## II. FIRST-PRINCIPLES CALCULATION OF JANUS MONOLAYER

Our first-principles calculations on monolayer MoSSe are conducted by using the projected augmented wave (PAW) method [3] implemented in the Vienna *ab initio* Simulation Package (VASP) [4, 5], based on density functional theory (DFT) [6, 7]. We adopt the generalized gradient approximation (GGA) with Perdew-Burke-Ernzerhof (PBE) scheme [8] for the exchange-correlation functional. The energy cut-off for the plane-wave is set to be 520 eV, and a $\Gamma$ centered $15\times15\times1$ $k$-mesh is adopted for the Brillouin zone sampling. The energy and force convergence threshold are set to be $10^{-6}$ eV and $10^{-3}$ eV/Å, respectively. A vacuum layer of 18 Å in the $z$-direction is added to avoid artificial interactions between periodic images. With the obtained DFT results, the maximally localized Wannier functions (MLWFs) are constructed by using the WANNIER90 package [9–11], with the $d$ orbitals of Mo and $p$ orbitals of S and Se atoms included. With the obtained ab-initio tight-binding model, the intrinsic NPHE response tensor is evaluated. In the calculation of $\chi^{\text{int}}$, a dense $\Gamma$-centered $k$-mesh with a spacing of 0.001 Å$^{-1}$ is adopted, and the temperature is set to be $T = 20$ K.


[1] D. Xiao, M.-C. Chang, and Q. Niu, Rev. Mod. Phys. **82**, 1959 (2010).
[2] Y. Gao, S. A. Yang, and Q. Niu, Phys. Rev. Lett. **112**, 166601 (2014).
[3] P. E. Blöchl, Phys. Rev. B **50**, 17953 (1994).
[4] G. Kresse and J. Hafner, Phys. Rev. B **49**, 14251 (1994).
[5] G. Kresse and J. Furthmüller, Phys. Rev. B **54**, 11169 (1996).
[6] P. Hohenberg and W. Kohn, Phys. Rev. **136**, B864 (1964).
[7] W. Kohn and L. J. Sham, Phys. Rev. **140**, A1133 (1965).
[8] J. P. Perdew, K. Burke, and M. Ernzerhof, Phys. Rev. Lett. **77**, 3865 (1996).
[9] N. Marzari and D. Vanderbilt, Phys. Rev. B **56**, 12847 (1997).
[10] I. Souza, N. Marzari, and D. Vanderbilt, Phys. Rev. B **65**, 035109 (2001).
[11] A. A. Mostofi, J. R. Yates, Y.-S. Lee, I. Souza, D. Vanderbilt, and N. Marzari, Comput. Phys. Commun. **178**, 685 (2008).
